# Supplementary material for: Generative Concatenative Nets Jointly Learn to Write and Classify Reviews
Source: arXiv:1511.03683 source file (2016-04-07)
Supplement: Supplementary file 1 [file classification-appendix.tex]

We trained a concatenated input RNN, 
with item category information as the auxiliary input. 
Inferring the class probability via the conditional likelihoods of the review, we can use the model \emph{in reverse}
to predict the category of the beer described in the review.
Using a balanced test set of 5000 reviews,
we evaluated the classification performance of
the category RNN against two softmax regression
classifiers, one trained on the top 10,000 n-grams
from the training set, and the other trained on
tf-idf transformed n-grams. 
The confusion matrices for these experiments can be seen in
\autoref{tab:confusion-catnet},
\autoref{tab:confusion-ngram},
and \autoref{tab:confusion-ngram-tfidf}.
We also show results for a generative concatenative network with rating information as used to classify positive ($\geq 4.0$ stars) and negative ($\leq 2.0$ stars) reviews.

\begin{table}[ht!]
\centering
  \begin{tabular}{|c | c |c c c c c|}
  \hline
  & & \multicolumn{5}{c|}{\textbf{Predicted Label}}\\
  \hline
  & & F/V & Lager & Stout & Porter & IPA \\
  \hline
  \multirow{5}{*}{\textbf{True Label}} 
  & F/V & 910 & 28  & 7  & 14  & 41 \\
  & Lager & 50  & 927 & 3   & 3  & 17 \\
  & Stout & 16   & 1   & 801 & 180 & 2  \\
  & Porter & 22   & 3   & 111  & 856 & 8\\
  & IPA & 19  & 12   & 4   & 12  & 953\\
  \hline
  \end{tabular}
\caption{Confusion matrix when classifying item category using the generative model in reverse.}
\label{tab:confusion-catnet}
\vspace{-15pt}
\end{table}

% [[ 910.   28.    7.   14.   41.]
%  [  50.  927.    3.    3.   17.]
%  [  16.    1.  801.  180.    2.]
%  [  22.    3.  111.  856.    8.]
%  [  19.   12.    4.   12.  953.]]

\begin{table}[ht!]
\centering
\begin{tabular}{|c |c |c c c c c|}
\hline
& & \multicolumn{5}{c|}{\textbf{Predicted Label}}\\
\hline
& & F/V & Lager & Stout & Porter & IPA \\
\hhline{-------}
\multirow{5}{*}{\textbf{True Label}} & F/V & 916 & 40 & 6 & 15 & 23\\
& Lager & 29 & 961 & 1 & 1 & 8\\
& Stout & 11 & 3 & 884 & 100 & 2\\
& Porter & 16 & 6 & 104 & 870 & 4\\
& IPA & 20 & 17 & 3 & 5 & 955\\
\hhline{-------}
\end{tabular}
\caption{Confusion matrix for item category classification with n-gram model.}
\label{tab:confusion-ngram}
\vspace{-15pt}
\end{table}

\begin{table}[ht!]
\centering
  \begin{tabular}{|c| c |c c c c c|}
  \hline 
  & & \multicolumn{5}{c|}{\textbf{Predicted Label}}\\
  \hline
  & & F/V & Lager & Stout & Porter & IPA \\
  \hhline{-------}
  \multirow{5}{*}{\textbf{True Label}} & F/V & 923 & 36 & 9 & 10 & 22\\
  & Lager & 16 & 976 & 0 & 1 & 7 \\
  & Stout & 9 & 4 & 920 & 65 & 2 \\
  & Porter & 11 & 6 & 90 & 887 & 6\\
  & IPA & 18 & 13 & 1 & 2 & 966 \\
  \hhline{-------}
  \end{tabular}
\caption{Confusion matrix for item category classification using n-gram tf-idf model.}
\label{tab:confusion-ngram-tfidf}
\vspace{-15pt}
\end{table}

\begin{table}[ht!]
\centering
  \begin{tabular}{|c| c |c c|}
  \hline 
  & & \multicolumn{2}{c|}{\textbf{Predicted Label}}\\
  \hline
  & & Negative & Positive \\
  \hline
  \multirow{2}{*}{\textbf{True Label}} & Negative &  294 & 206 \\
  & Positive & 7 & 493\\
  \hline
  \end{tabular}
\caption{Positive($\geq 4$ stars)/ negative ($\leq 2$ stars.) classification results for RNN }
\label{tab:confusion-rat-ratnet}
\vspace{-15pt}
\end{table}

% [[294 206]
%  [  7 493]]

\begin{table}[ht!]
\centering
  \begin{tabular}{|c| c |c c|}
  \hline 
  & & \multicolumn{2}{c|}{\textbf{Predicted Label}}\\
  \hline
  & & Negative & Positive \\
  \hline
  \multirow{2}{*}{\textbf{True Label}} & Negative &  464 & 36\\
  & Positive & 191 & 309\\
  \hline
  \end{tabular}
\caption{n-gram tf-idf positive/negative classification results trained without balancing dataset.}
\label{tab:confusion-rat-train-ngram-tfidf}
\vspace{-15pt}
\end{table}

\begin{table}[ht!]
\centering
  \begin{tabular}{|c| c |c c|}
  \hline 
  & & \multicolumn{2}{c|}{\textbf{Predicted Label}}\\
  \hline
  & & Negative & Positive \\
  \hline
  \multirow{2}{*}{\textbf{True Label}} & Negative &  459 & 41\\
  & Positive & 42 & 458\\
  \hline
  \end{tabular}
\caption{n-gram tf-idf positive/negative classification results on balanced dataset.}
\label{tab:confusion-rat-ngram-tfidf}
\vspace{-10pt}
\end{table}
